# Supplementary material for: Multi-Objective SPIBB: Seldonian Offline Policy Improvement with Safety Constraints in Finite MDPs
Source: arXiv:2106.00099 source file (2021-10-29)
Supplement: Supplementary file 1 [file spibb_extra_details.tex]

\section{SPIBB formulation details}
\label{app:spibb-background}

% ------------------------------------------------------
%                       SPIBB 
% ------------------------------------------------------

% An alternate objective that might be of interest is the following: 
% \begin{align}
%     \max_{\pi} &\quad J(\pi, \hat{M}) \label{eq:alt-batch-pi}\\ 
%     \texttt{s.t.} &\quad J(\pi, M) \geq J(\pi_b, M) - \xi, \forall M \in \Xi,
%     \nonumber \\
%     &\quad J(C_i, \pi, \hat{M}) \leq d_i, \forall i, \nonumber \\
%     &\quad J(C_i, \pi, M) \leq f(d_i, \xi), \forall i. \nonumber
% \end{align}

% The main difference between Eq.~\ref{eq:batch-pi} and Eq.~\ref{eq:alt-batch-pi} is that in Eq.~\ref{eq:alt-batch-pi} the constraint satisfaction is a hard constraint with respect to the estimated MDP, and for constraint satisfaction in the admissible MDPs we would like it to be some function of $\xi$-like quantity (to be decided). 

% \harsh{Hypothesis: One of the problems with the CMDPs formulation is that sometimes the algorithms finds the solution that is just below the constraint threshold. While this is okay in certain scenarios it ends up being more like a equality constraint. In this scenario, user can specify that the goal is to increase safety/reduce constraints, while making sure the performance doesn't suffer much.}

The SPIBB algorithm \citep{laroche2017safe} takes input a dataset of trajectories under the baseline policy $\D$, as well as needs access to the baseline policy $\pib$ to do return a improved policy based on the guarantees parameters provided by the user.

The high level methodology of the SPIBB algorithm is along the following lines. The first step is to  build a bootstrap set $\Bset$, a set of state-action pairs with counts less than $N_\Lambda$ (hyper-parameter). When the state-action pair has low confidence (rarely encountered in the dataset), SPIBB will bootstrap the baseline policy for it. Here bootstrapping means that the agent will rely on the baseline policy and copy the probabilities for that state-action pair, 
\begin{equation*}
    \pi^{\odot}_{spibb}(a|x) = \pi_b(a|x) \text{ if } (x,a) \in \Bset.
\end{equation*}
For the non-bootstrapped actions, SPIBB uses the greedy update but restricted to the non-bootstrapped actions:
\begin{equation*}
    \pi^{(i)}_{spibb}(x , \argmax_{a \mid a \notin \Bset} Q^{(i)}(x,a)) = \sum_{a \mid a \notin \Bset} \pi_b(a|x)
\end{equation*}
SPIBB is based on the binary classification of the bootstrapped set: either a pair either belongs to it and cannot affect the new policy, or it does not and the policy is changed completely for that pair. 

In Soft-SPIBB \citep{nadjahi2019safe}, authors  the objective that allows slight policy changes for uncertain state-action pairs while remaining safe. The authors constrain the class of policies to $(\pi_b, e, \epsilon)$-constrained policies: 
\begin{equation}
    \sum_a e(x,a)\ |\pi(a|x) - \pi_{b}(a|x)| \leq \epsilon,  \forall x \in \X,
\end{equation}
where $e: \X \times \A \rightarrow \Real$ is an error function on the state-action value function $Q$ and $\epsilon$ is a hyper-parameter that controls the deviation from the baseline policy. The second constraint is to improve the performance of the new policy w.r.t. the baseline, i.e. to a find $\pi_b$-advantageous policy:
\begin{equation}
\label{eq:spibb-performance-constraint}
\sum_a \pi(a|x) A^{\pi_b}(x, a) \geq 0, \forall x \in \X,
\end{equation}
where $A^{\pi_b}$ denotes the advantage function: $A^{\pi}(x,a) = Q^{\pi}(x,a) - V^{\pi}(x)$. Under these two conditions, i.e., if the policy is $\pi_b$-advantageous and $(\pi_b, e_Q, \epsilon)$-constrained then it is possible to show  can have the safety guarantees.  The new policy improvement can be viewed as:
    \begin{align}
        \label{eq:soft-spibb-obj}
        \pi_{new} &= \argmax_{\Pi} \langle \pi(\cdot|x) Q^{\pi_b}(x,\cdot) \rangle \quad \forall x \in \X  \\
        \texttt{s.t.} &\sum_a e_Q(x,a)\ |\pi(a|x) - \pi_{b}(a|x)| \leq \epsilon, \nonumber \\ 
        &\sum_a \pi(a|x) = 1 . \nonumber
    \end{align}

% more details
As such they are working with a constrained optimization problem/LP, that they propose to solve in every iteration of the policy improvement. The exact solution of the LP can be found with simplex or mixed integer programming. The authors also propose an approximate method for calculating the solution.
However, these policy constraints can be too conservative, they use $e_P$, to relax the policy space and use another assumption to guarantee safety bounds.
