# Supplementary material for: Multi-Objective SPIBB: Seldonian Offline Policy Improvement with Safety Constraints in Finite MDPs
Source: arXiv:2106.00099 source file (2021-10-29)
Supplement: Supplementary file 2 [file error_bounds.tex]

\section{Error bounds}
\label{app:err-bounds}

Using the same notation from \cite{nadjahi2019safe}, we have:

\begin{align}
    \norm{P(.|x,a) - \hat{P}(.|x,a)}_{1} &\leq e_P(x,a),  \label{eq:eP}
    \\ \abs{R(x,a) - \hat{R}(x,a)} &\leq e_P(x,a) R_{\max}, \label{eq:eR}
    \\ \abs{C_i(x,a) - \hat{C_{i}}(x,a)} &\leq e_P(x,a) C_{i_{\max}}, \quad (\forall i),   \label{eq:eC}
    \\ \abs{Q^{\pi_b}_{M*}(x,a) - Q^{\pi_b}_{\hat{M}}(x,a)} &\leq e_Q(x,a) V_{\max},  \label{eq:eQ}
    \\ \abs{{Qc}^{\pi_b}_{i, M*}(x,a) - Q^{\pi_b}_{i, \hat{M}}(x,a)} &\leq e_Q(x,a) {Vc}_{\max},  \label{eq:eQc}
\end{align}
where,
\begin{align}
    e_P(x,a) &= \sqrt{\frac{2}{N_{\D}(x,a)} \log\frac{2 \abs{\X}\abs{A}2^{\abs{\X}}}{\delta}}, 
    \\ e_Q(x,a) &= \sqrt{\frac{2}{N_{\D}(x,a)} \log\frac{2 \abs{\X}\abs{A}}{\delta}}.
\end{align}
